# Supplementary material for: Active Learning with Selective Time-Step Acquisition for PDEs
Source: arXiv:2511.18107 source file (2026-04-16)
Supplement: Supplementary file 1 [file batch.tex]

\section{Justification for Cost of a batch}
\label{app:cost_justification}

Sometimes, we are given a batched numerical solver that is more efficient when solving for $N$ queries simulataneously, rather than solving for them one at a time. In that case, one might wonder if the cost of acquiring a batch really is the number of time steps. For instance, if we were to acquire a trajectory of length $L$, the solver would have to be run sequentially, $L$ times. On the other hand, if we were to acquire one time step each from $L$ different trajectories, we could run the solver in parallel only once. Suppose that, up to a certain threshold number of queries $N$, solving for them in parallel takes constant time. We prove that the cost of a batch is indeed the total number of time steps, if the number is equal to $N \times L$.

This is due to Gale-Ryser theorem, which provides sufficient conditions under which there exists a binary matrix with prescribed row and column sums. In this context, the trajectories correspond to the row, with the $j^\text{th}$ trajectory requiring a sequence of $n_j$ time steps. The batches that are queried simultaneously correspond to the columns, with each batch capable of processing up to $N$ time steps simultaneously. The total number of time steps is $\sum_j n_j  = N \times L$, and the theorem ensures that we can schedule these steps into exactly $L$ batches, each processing $N$ time steps. Specifically, since the row sums $n_j $ do not exceed $ L$, the maximum possible sum of the top $k$ row sums is $k\times L$, and . Hence, the cost of acquiring a batch across multiple trajectories is indeed equivalent to the total number of time steps $N \times L$, validating the efficiency of the batched numerical solver.

Therefore, the budget size should ideally be set to $ N\times L$, where $N$ depends on the current solver and hardware. Although our toy benchmarks have a large $N$ due to their small complexity, we pretended as if $N=8$ in our experiments, since we want our method to be applicable to more complex tasks.
